# Supplementary material for: Widening Access to Applied Machine Learning with TinyML
Source: arXiv:2106.04008 source file (2021-06-09)
Supplement: Supplementary file 1 [file 12appendix.tex]

\section{Appendix}
TinyML on edX is designed in five chapters across four courses. For the most up-to-date details and for links to all slides, readings, and Colab notebooks, visit our courseware Github: \href{https://github.com/tinyMLx/courseware}{\texttt{https://github.com/tinyMLx/courseware}}.
